# Supplementary material for: Characterizing Individual Communication Patterns
Source: arXiv:0905.0106 source file (2009-05-01)
Supplement: Supplementary file 1 [file appendix.tex]

%==============================================================================
%==============================================================================
%==============================================================================
% APPENDIX
%==============================================================================
%==============================================================================
%==============================================================================
\appendix

%==============================================================================
%==============================================================================
%==============================================================================
% PARAMETER ESTIMATION
%==============================================================================
%==============================================================================
%==============================================================================
\section{Parameter estimation}

% introduction to this section
Estimating the parameters $\bftheta$ of our model for human activity is
complicated by the fact that the time series data are left- and right-censored.
That is, given a set of $\N$ ordered events $\{\tn{1}, \tn{2}, \dots,\tn{\N}\}$
for a particular individual, we wish to estiamte the parameters $\bftheta$ over
a finite time interval $[\tn{0},\tn{\N+1})$ where $\tn{0}<\tn{1}< \cdots <
\tn{\N} < \tn{\N+1}$.  We denote this set of known observations as $\T =
\{\tn{0},\dots,\tn{\N+1}\}$.  Before describing the inference process for our
double-chain Markov model, it is fruitful to first describe the inference
procedure for left- and right-censored data sets with simpler models.

% non-hidden Poisson processes (homogeneous then non-homogeneous)
Consider a homogeneous Poisson process with constant rate $\rate$.  For a
homogeneous Poisson process, there is a constant probability $\rate\dt$ that an
event occurs during the infinitesimally small time interval $[\ttt,\ttt+\dt)$
and, as a result, the complete data likelihood is given by
\begin{eqnarray}
  \condprob{\T}{\rate} \mul \dt^{N} & = & 
  \left[\prod_{\n=1}^{\N} (1-\rate\dt)^{(\tn{\n}-\tn{\n-1})/\dt-1} \mul\rate\dt \right]
  \mul (1-\rate\dt)^{(\tn{\N+1}-\tn{\N})/\dt-1} \nonumber \\
  & = & 
  \left[\prod_{\n=1}^{\N} e^{-\rate (\tn{\n} - \tn{\n-1})} \mul \rate\dt \right]
  \mul  e^{-\rate (\tn{\N+1} - \tn{\N})} 
\end{eqnarray}
or
\begin{eqnarray}
  \condprob{\T}{\rate} & = & 
  \left[\prod_{\n=1}^{\N} \condprob{\deltat=\tn{\n}-\tn{\n-1}}{\tn{\n-1},\rate} \right]
  \mul  \condprob{\deltat>\tn{\N+1}-\tn{\N}}{\tn{\N},\rate}
\end{eqnarray}
It is straightforward to confirm the intuitive result that the best-estimate
rate $\widehat{\rate}=\N/(\tn{\N+1}-\tn{0})$.  Extending this result to a
non-homogeneous Poisson process with rate $\rate(\ttt)$, one obtains
\begin{eqnarray}
  \condprob{\T}{\rate(\ttt)} & = & 
  \left[\prod_{\n=1}^{\N} \condprob{\deltat=\tn{\n}-\tn{\n-1}}{\tn{\n-1},\rate(\ttt)} \right]
  \mul  \condprob{\deltat>\tn{\N+1}-\tn{\N}}{\tn{\N},\rate(\ttt)}
\end{eqnarray}
which can be maximized numerically to compute $\widehat{\rate}(\ttt)$.  

% double-chain Markov process
In our particular case, however, we believe that each inter-event time
$\deltat$ is drawn from either a non-homogeneous Poisson process or a
homogeneous Poisson process depending on whether the individual is between
active intervals or within an active interval, respectively
(\figref{\ref{fig:likelihood}}).  We adopt the notation of
Bishop~\cite{bishop07} and denote the state of the individual at time $\tn{\n}$
by the vector $\zn{\n}$ where $\prob{\znk{\n\kk=1}}$ denotes the probability
that the individual is in state $\kk$ at time $\tn{\n}$.  We can incorporate
this knowledge in the complete data likelihood function given by
\begin{eqnarray}
\condprob{\T,\Z}{\bftheta} & = & 
  \condprob{\deltat=\tn{1}-\tn{0}}{\tn{0},\zn{1},\bftheta} \mul
  \condprob{\zn{1}}{\bftheta} \times \nonumber \\ & &
  \left[\prod_{\n=2}^{\N}
    \condprob{\deltat=\tn{\n}-\tn{\n-1}}{\tn{\n-1},\zn{\n},\bftheta} 
    \mul \condprob{\zn{\n}}{\zn{\n-1},\bftheta} \right] \times \nonumber \\
  & & \mul \condprob{\deltat>\tn{\N+1}-\tn{\N}}{\tn{\N},\zn{\N+1},\bftheta} 
      \mul \condprob{\zn{\N+1}}{\zn{\N},\bftheta} .
\end{eqnarray}
We can then compute the best-estimate parameters $\widehat{\bftheta}$ of this
double-chain Markov model with a slight modification of the
expectation-maximization (EM) algorithm for a standard hidden Markov
model~\cite{bishop07}.  

%==============================================================================
% FORWARD-BACKWARD
%==============================================================================
\subsection{Expectation step}

During the E-step, we use forward-backward recursion to
compute $\condprob{\Z}{\T,\bfthetaold}$ based on some initial parameter guess
$\bfthetaold$.  We first define
\begin{eqnarray}
\gn{\n} & = & \condprob{\zn{\n}}{\T} \nonumber \\ 
        & = & \frac{\condprob{\T}{\zn{\n}}\mul\prob{\zn{\n}}}{\prob{\T}} \nonumber \\
        & = & \frac{\prob{\T,\zn{\n}}}{\prob{\T}} \nonumber \\
        & = & \frac{\prob{\tn{0},\dots,\tn{\n},\zn{\n}}\mul
                    \condprob{\tn{\n+1},\dots\tn{\N+1}}{\tn{\n},\zn{\n}}}{\prob{\T}} 
              \nonumber \\
        & = & \frac{\an{\n}\mul\bn{\n}}{\prob{\T}}
\end{eqnarray}
and 
\begin{eqnarray}
\xn{\n-1}{\n} & = & \condprob{\zn{\n-1},\zn{\n}}{\T} \nonumber \\
             & = & \frac{\condprob{\T}{\zn{\n-1},\zn{\n}} \mul 
                         \prob{\zn{\n-1},\zn{\n}}}
                        {\prob{\T}} \nonumber \\
             & = & \frac{\condprob{\tn{0},\dots,\tn{\n-1}}{\zn{\n-1},\zn{\n}}
                         \mul
                         \condprob{\tn{n}}{\tn{\n-1},\zn{\n-1},\zn{\n}} 
                         \mul
                         \condprob{\tn{n+1},\dots,\tn{\N+1}}{\tn{\n},\zn{\n-1},
                                                           \zn{\n}}
                         \mul
                         \condprob{\zn{\n}}{\zn{\n-1}} \mul \prob{\zn{\n-1}}}
                        {\prob{\T}} \nonumber \\
             & = & \frac{\condprob{\tn{0},\dots,\tn{\n-1}}{\zn{\n-1}}
                         \mul
                         \condprob{\tn{n}}{\tn{\n-1},\zn{\n}} 
                         \mul
                         \condprob{\tn{n+1},\dots,\tn{\N+1}}{\tn{\n},
                                                             \zn{\n}}
                         \mul
                         \condprob{\zn{\n}}{\zn{\n-1}} \mul \prob{\zn{\n-1}}}
                        {\prob{\T}} \nonumber \\
             & = & \frac{\prob{\tn{0},\dots,\tn{\n-1},\zn{\n-1}}
                         \mul
                         \condprob{\tn{n}}{\tn{\n-1},\zn{\n}} 
                         \mul
                         \condprob{\tn{n+1},\dots,\tn{\N+1}}{\tn{\n},
                                                           \zn{\n}}
                         \mul
                         \condprob{\zn{\n}}{\zn{\n-1}}}
                        {\prob{\T}} \nonumber \\
             & = & \frac{\an{\n}
                         \mul
                         \condprob{\tn{n}}{\tn{\n-1},\zn{\n}} 
                         \mul
                         \bn{\n}
                         \mul
                         \condprob{\zn{\n}}{\zn{\n-1}}}
                        {\prob{\T}} \;.
\end{eqnarray}
Both $\gn{\n}$ and $\xn{\n-1}{\n}$ depend only on
$\condprob{\tn{\n}}{\tn{\n-1},\zn{\n}}$ and $\condprob{\zn{\n}}{\zn{\n-1}}$
which are defined by our model and $\an{\n}$ and $\bn{\n}$ which are computed
by forward-backward recursion:
\begin{eqnarray}
\an{\n} & = & \prob{\tn{0},\dots,\tn{\n},\zn{\n}} \nonumber \\
        & = & \condprob{\tn{\n}}{\tn{0},\dots,\tn{\n-1},\zn{\n}} 
              \mul
              \prob{\tn{0},\dots,\tn{\n-1},\zn{\n}} \nonumber \\
        & = & \condprob{\tn{\n}}{\tn{\n-1},\zn{\n}} 
              \mul
              \prob{\tn{0},\dots,\tn{\n-1},\zn{\n}} \nonumber \\
        & = & \condprob{\tn{\n}}{\tn{\n-1},\zn{\n}} 
              \mul
              \sum_{\zn{\n-1}}\prob{\tn{0},\dots,\tn{\n-1},\zn{\n-1},\zn{\n}} \nonumber \\
        & = & \condprob{\tn{\n}}{\tn{\n-1},\zn{\n}} 
              \mul
              \sum_{\zn{\n-1}}\prob{\tn{0},\dots,\tn{\n-1},\zn{\n-1}} 
                            \mul \condprob{\zn{\n}}{\zn{\n-1}} \nonumber \\
        & = & \condprob{\tn{\n}}{\tn{\n-1},\zn{\n}} 
              \mul
              \sum_{\zn{\n-1}}\an{\n-1}
                            \mul \condprob{\zn{\n}}{\zn{\n-1}} \nonumber \\
\end{eqnarray}
where $\an{1} = \bfpi$ and 
\begin{eqnarray}
\bn{\n} & = & \condprob{\tn{\n+1},\dots,\tn{\N+1}}{\tn{\n},\zn{\n}} \nonumber \\
        & = & \sum_{\zn{\n+1}} \condprob{\tn{\n+1},\dots,\tn{\N+1},\zn{\n+1}}
                                      {\tn{\n},\zn{\n}} 
              \nonumber \\
        & = & \sum_{\zn{\n+1}} \condprob{\tn{\n+1},\dots,\tn{\N+1}}
                                      {\tn{\n},\zn{\n},\zn{\n+1}}
                             \mul
                             \condprob{\zn{\n+1}}{\tn{\n},\zn{\n}}
              \nonumber \\
        & = & \sum_{\zn{\n+1}} \condprob{\tn{\n+1},\dots,\tn{\N+1}}
                                      {\tn{\n},\zn{\n+1}}
                             \mul
                             \condprob{\zn{\n+1}}{\zn{\n}}
              \nonumber \\
        & = & \sum_{\zn{\n+1}} \condprob{\tn{\n+1}}
                                      {\tn{\n},\zn{\n+1}}
                             \mul
                             \condprob{\tn{\n+2},\dots,\tn{\N+1}}
                                      {\tn{\n},\zn{\n+1}}
                             \mul
                             \condprob{\zn{\n+1}}{\zn{\n}}
              \nonumber \\
        & = & \sum_{\zn{\n+1}} \condprob{\tn{\n+1}}
                                      {\tn{\n},\zn{\n+1}}
                             \mul
                             \bn{\n+1}
                             \mul
                             \condprob{\zn{\n+1}}{\zn{\n}}
\end{eqnarray}
where $\bn{\N+1} = 1$.  

%==============================================================================
% MAXIMIZATION STEP
%==============================================================================
\subsection{Maximization step}

During the M-step, we wish to maximize 
%% %
%% \begin{eqnarray}
%% \condprob{\bftheta}{\T} & = & \frac{\condprob{\T}{\bftheta} 
%%                                     \mul \prob{\bftheta}}
%%                                    {\prob{\T}} \nonumber \\
%%                         & = & \frac{\sum_{\Z}\condprob{\T,\Z}{\bftheta}
%%                                     \mul \prob{\bftheta}}
%%                                    {\sum_{\Z} \prob{\T,\Z}} \nonumber \\
%%                         & \propto & \sum_{\Z}\condprob{\T,\Z}{\bftheta}
%% \label{eqn:Q}
%% \end{eqnarray}
%% %
%
\begin{eqnarray}
\mathcal{Q}(\bftheta,\bfthetaold) & = & \sum_{\Z} \condprob{\Z}{\T,\bfthetaold} 
                                        \mul
                                        \ln \condprob{\T,\Z}{\bftheta}
\label{eqn:Q}
\end{eqnarray}
with respect to the parameters $\bftheta = \{ \bfpi, \bfA, \bfphi\}$ to update
our best estimate parameters $\widehat{\bftheta}$ from our previous
best-estimate of the parameters $\bfthetaold$.  Given the double-chain Markov
structure of our model, the complete-data likelihood is given by
\begin{eqnarray}
\condprob{\T,\Z}{\theta} & = & \condprob{\zn{1}}{\bfpi} \mul
                               \left[ \prod_{\n=2}^{\N+1} 
                                      \condprob{\zn{\n}}{\zn{\n-1},\bfA} 
                               \right] \mul
                               \left[ \prod_{\n=1}^{\N+1} 
                                      \condprob{\tn{\n}}
                                               {\tn{\n-1},\zn{\n},\bfphi} 
                               \right] \;. 
\label{eqn:complete_likelihood}
\end{eqnarray}
After
substituting \eqnref{\ref{eqn:complete_likelihood}}~into \eqnref{\ref{eqn:Q}},
we obtain
\begin{eqnarray}
\mathcal{Q}(\bftheta,\bfthetaold) & = & \sum_{\Z} \condprob{\Z}{\T,\bfthetaold} 
                                        \mul
                                        \ln \condprob{\zn{1}}{\bfpi} 
                                        \nonumber \\
                                  & & + \sum_{\Z} \condprob{\Z}{\T,\bfthetaold} 
                                        \mul
                                        \ln \condprob{\zn{\n}}{\zn{\n-1},\bfA}
                                        \nonumber \\
                                  & & + \sum_{\Z} \condprob{\Z}{\T,\bfthetaold} 
                                        \mul
                                        \ln \condprob{\tn{\n}}
                                                     {\tn{\n-1},\zn{\n},\bfphi} 
                                        \nonumber \\
                                  & = & \sum_{\kk=1}^{\K} \gnk{1 \kk}
                                        \mul
                                        \ln \pik{\kk}
                                        \nonumber \\
                                  & & + \sum_{\n=2}^{\N+1} \sum_{\jj=1}^{\K} 
                                        \sum_{\kk=1}^{\K} \xnk{\n-1,\jj}{\n \kk}
                                        \mul
                                        \ln \Ajk{\jj \kk}
                                        \nonumber \\
                                  & & + \sum_{\n=1}^{\N+1} \sum_{\kk=1}^{\K} 
                                        \gnk{\n \kk}
                                        \mul
                                        \ln \condprob{\tn{\n}}
                                                     {\tn{\n-1},\znk{\n \kk},\bfphi} \;.
\label{eqn:Q2}
\end{eqnarray}
Due to the separability of \eqnref{\ref{eqn:Q2}}~and the fact that our model
only has $K=2$ latent states, it is straightforward to show that 
\begin{eqnarray}
\hat{\pik{\kk}} & = & \frac{\gnk{1 \kk}}{\sum_{\jj=1}^{\K} \gnk{1 \jj}} \;.
\end{eqnarray}
To find the best-estimate $\widehat{\bfA}$, it is worth noting that $\bfA$ is
parameterized by a single parameter, $\qq$---the probability of starting a new
active interval.  So, if state $\znk{\n 1}=1$ denotes starting a new active
interval, 
\begin{eqnarray}
\bfA & = & 
\begin{pmatrix}
1-\qq & \qq \\
1-\qq & \qq
\end{pmatrix}
\end{eqnarray}
and 
\begin{eqnarray}
\widehat{\qq} & = & \frac{\sum_{\n=2}^{\N+1} \sum_{\jj=1}^{\K} \xnk{\n-1, \jj}{\n 2}} 
                         {\sum_{\n=2}^{\N+1} \sum_{\jj=1}^{\K} \sum_{\kk=1}^{\K} 
                          \xnk{\n-1, \jj}{\n \kk}} \; .
\end{eqnarray}
Finally, obtaining the best-estimate $\widehat{\bfphi}$ reduces to numerically
maximizing the third term of \eqnref{\ref{eqn:Q2}}.
